# Supplementary material for: Semantics-Guided Synthesis
Source: arXiv:2008.09836 source file (2020-11-11)
Supplement: Supplementary file 1 [file additional-eval.tex]

\section{Additional Evaluation}
\label{Se:AdditionalEval}

\input{resulttable}
